# Supplementary material for: Accelerating materials discovery for polymer solar cells: Data-driven insights enabled by natural language processing
Source: arXiv:2402.19462 source file (2024-06-22)
Supplement: Supplementary file 1 [file A-Appendix.tex]

\section{Appendix}
